# Supplementary material for: Active Visuo-Tactile Point Cloud Registration for Accurate Pose Estimation of Objects in an Unknown Workspace
Source: arXiv:2108.04015 source file (2021-08-09)
Supplement: Supplementary file 2 [file appendix_old.tex]

\appendices
\label{sec:appendix}
\section{Mathematical Notation}
The mathematical notation and formulations used in the paper is detailed below:
\begin{itemize}
    \item Let $p \in \mathbb{R}^3$ denote a 3D column vector representing a point in $\mathbb{R}^3$.
    \item Let ${}^A H_B \in \mathbb{R}^{4 \times 4}$ be the homogeneous transformation matrix describing the transformation of a point from the frame B to the frame A. ${}^A H_B = \begin{bmatrix} {}^A R_B & {}^A o_B \\  0_{1\times 3} & 1 \end{bmatrix}$ where ${}^A R_B$ is the rotation matrix and ${}^A o_B$ is the translation vector of frame B with respect to frame A.
    \item Let $\hat{\mathbf{q}}$ denote a general quaternion, where $\mathbf{q}$ refers to the vector component of the quaternion and $q_0$ to the real part such that $\hat{\mathbf{q}} = [q_{0}, \mathbf{q}^T]^T$. Basic operations on quaternions is defined as follows:
    \begin{itemize}
        \item Scalar multiplication with a quaternion is given by: $s \hat{\mathbf{q}} = [s q_{0}, s\mathbf{q}^T]^T$.
        \item Addition of two quaternions is given by: $\hat{\mathbf{q}}_1 + \hat{\mathbf{q}}_2 = [q_{0_1} + q_{0_2}, (\mathbf{q}_1 + \mathbf{q}_2)^T]^T$.
        \item Multiplication of two quaternions is given by: 
        \begin{equation}
        \begin{aligned}
            \hat{\mathbf{q}}_1 \odot \hat{\mathbf{q}}_2  
            &= \begin{bmatrix}
            q_{0_1} & -\mathbf{q_1}^T \\ \mathbf{q_1} & \mathbf{q_1}^{\times} + q_{0_1}\mathbb{I}_3  
            \end{bmatrix}\hat{\mathbf{q}}_2 \quad , \\
            &= \begin{bmatrix}
            q_{0_2} & -\mathbf{q_2}^T \\ \mathbf{q_2} & \mathbf{q_2}^{\times} - q_{0_2}\mathbb{I}_3  
            \end{bmatrix}\hat{\mathbf{q}}_1 \quad ,
        \end{aligned}
        \label{eq:quaternionmult}
        \end{equation}
        where $\odot$ is the quaternion multiplication operator and $[v]^{\times}$ is the skew-symmetric matrix formed from the vector $v$.
        \item Conjugate $\hat{\mathbf{q}^{*}}$ is given by $\hat{\mathbf{q}^{*}} = [q_0, -\mathbf{q^T}]$.
        \item The norm of a quaternion is $|\hat{\mathbf{q}}| = \sqrt{scalar(\hat{\mathbf{q}}\odot \hat{\mathbf{q}^*})}$ and a unit quaternion is one with $|\hat{\mathbf{q}}| = 1$.
    \end{itemize}
\end{itemize}


% \section{Notation}

% \subsection{Quaternions}
% We denote a general quaternion as $\hat{\mathbf{q}}$, where $\mathbf{q}$ refers to the vector component of the quaternion and $q_0$ to the real part.
% \begin{equation}
%     \hat{\mathbf{q}} = [q^{(0)}, \mathbf{q}^T]^T
% \end{equation}
% We show a few important arithmetic operations: 

% Scalar Multiplication
% \begin{equation}
%     s \hat{\mathbf{q}} = [s q^{(0)}, s\mathbf{q}^T]^T
% \end{equation}

% Addition
% \begin{equation}
%     \hat{\mathbf{q}}_1 + \hat{\mathbf{q}}_2 = [q^{(0)}_{1} + q^{(0)}_{2}, (\mathbf{q}_1 + \mathbf{q}_2)^T]^T
% \end{equation}

% Multiplication
% \begin{equation}
%     \hat{\mathbf{q}}_1 \odot \hat{\mathbf{q}}_2 = [q^{(0)}_{1}\cdot q^{(0)}_{2} - \mathbf{q}_1^T \cdot \mathbf{q}_2, (q^{(0)}_{1}\mathbf{q}_2 + q^{(0)}_{2}\mathbf{q}_2 +  \mathbf{q}_1 \times \mathbf{q}_2)^T]^T
% \end{equation}

% \subsection{Dual Numbers}
% Dual Numbers are a concept similar to complex numbers. A dual number $z$ is defined as 
% \begin{equation}
%     z = r + \epsilon d
% \end{equation}
% with $r$ being the real part and $d$ the dual part. The dual operator $\epsilon$ has the constraints $\epsilon \neq 0$ and $\epsilon^2 = 0$.
% This notation has its own arithmetics:

% Addition
% \begin{equation}
%     z_1 + z_2 = (r_1 + r_2) + \epsilon (d_1 + d_2)
% \end{equation}

% Multiplication
% \begin{equation}
%     z_1 \otimes z_2 = (r_1 + \epsilon d_1) \otimes (r_2 + \epsilon d_2) = (r_1\cdot r_2) + \epsilon(r_1 \cdot d_2 + r_2 \cdot d_1)
% \end{equation}
% The dual-product is given its own symbol $\otimes$ to make it more simple to follow derivations.

% \subsection{Dual Quaternions}
% Dual-numbers also generalize to quaternions. Dual-quaternions are defined as
% % \begin{equation}
    
% % \end{equation}

% \section{Dual Quaternions}
% TBD

% \section{From Dual Quaternions to Translation invariant Measurements}

% Given a point from our model $\mathbf{b}$ and a point of contact that is measured with the tactile sensor $\mathbf{a}$ we can formulate the relation
% \begin{equation}
%     \mathbf{a} = \mathbf{R} \mathbf{b} + \mathbf{t}
% \end{equation}

% Where $\mathbf{R}\in SO(3)$ is a rotation matrix and $t\in \mathbb{R}^3$ is a translation vector. Note that we assume no noise up to now. This relation holds for all corresponding points in the model and the measurements. We can express the same equation using dual-quaternions as
% \begin{equation}
%     \hat{\mathbf{a}} = \hat{\mathbf{d}}\otimes \hat{\mathbf{b}} \otimes \hat{\mathbf{d}}^{3*} 
% \end{equation}
% Hat denotes a quaternion, 
